# Supplementary material for: VIC: Evasive Video Game Cheating via Virtual Machine Introspection
Source: arXiv:2502.12322 source file (2025-02-21)
Supplement: Supplementary file 1 [file appendix.tex]

\appendix
